# Supplementary material for: From Lazy to Prolific: Tackling Missing Labels in Open Vocabulary Extreme Classification by Positive-Unlabeled Sequence Learning
Source: arXiv:2408.08981 source file (2025-01-09)
Supplement: Supplementary file 1 [file appendix_wiki_main.tex]

\setlength{\tabcolsep}{4pt}
\begin{table*}[!t]
\centering
\scriptsize
% \begin{tabular}{@{}rrrrrrrrrrrrrrr@{}}
\begin{tabular}{@{}lllllllllllllll@{}}

\toprule
                             & \multicolumn{14}{c}{Wikipedia-1M ($\mu=5, \text{CV}=0.9$)}                                                                                                                                                                                               \\ \midrule
\multicolumn{1}{c|}{}        & \multicolumn{7}{c|}{Narrow ($|Y| \leq 2\mu$) (91.0\%)}                                                                     & \multicolumn{7}{c}{Diverse ($ |Y| > 2\mu$) (8.9\%)}                                               \\ \midrule
\multicolumn{1}{l|}{}        & P@$\mathcal{O}$ & R@$\mathcal{O}$ & F1@$\mathcal{O}$ & B@$\mu$ & \#K@$\mu$ & B@$2\mu$ & \multicolumn{1}{c|}{\#K@$2\mu$} & P@$\mathcal{O}$ & R@$\mathcal{O}$ & F1@$\mathcal{O}$ & B@$\mu$ & \#K@$\mu$ & B@$2\mu$ & \#K@$2\mu$ \\ \midrule
\multicolumn{1}{l|}{One2One} &         \underline{34.23}&       \underline{34.18}&       \underline{34.2}&    \underline{29.75}&    -&    \textbf{20.60}& \multicolumn{1}{l|}{-}           &             38.24    &      \textbf{38.04}&       38.13           &  \underline{57.80}&     -&     \textbf{45.94}&     -\\
\multicolumn{1}{l|}{GROOV}   &     \textbf{67.04}&   \textbf{45.18}&   \textbf{52.02}&   \textbf{31.13}&    2.30       &   \underline{15.60}& \multicolumn{1}{l|}{2.31}           &     \textbf{84.79}&    26.24             &       \underline{39.2}&    \textbf{67.66}&    3.94       &    36.00      &    4.22        \\
\multicolumn{1}{l|}{One2Seq} &     23.50            &   19.91              &     21.15             &   17.69      &    3.85       &    11.27      & \multicolumn{1}{l|}{5.79}           &      \underline{45.97}&    34.76             &     38.61             &     52.85    &    4.66       &    40.16      &       8.17     \\
\multicolumn{1}{l|}{PUSL}    &      21.18          &     19.09           &     19.81             &    17.54     &     \textbf{3.99}&     11.71     & \multicolumn{1}{l|}{\textbf{6.26}}           &           45.08      &         \underline{37.89}&      \textbf{40.37}&   53.96      &   \textbf{4.79}&     \underline{42.94}&    8.75        \\
% \midrule
\bottomrule
\end{tabular}
\caption{Evaluation results on Wiki-IID test splits}
\label{tab:wiki_iid}
\end{table*}
